# Supplementary material for: Hallucinating Agnostic Images to Generalize Across Domains
Source: arXiv:1808.01102 source file (2019-07-10)
Supplement: Supplementary file 1 [file appendix.tex]

\textbf{Residual Transformer} We provide here some more information on the residual transformer that we used as reference module when building \our. 

In Figure \ref{fig:transformer_residual} we present its architecture: note that the choice of adding the last residual operation that combines the original image with the intermediate residual block output was not used in \cite{carlucci2018text} and is introduced here to help the whole network stability.  We tested some variations of this architecture by augmenting or reducing  the number of filters and the number of residual blocks, observing small performance variations so we decided to keep the original structure.

In Table \ref{table:ablation3} we complete the ablation study showing the results obtained with the residual transformer. As already indicated in the main paper, the behavior of the residual $T$ in combination with the other modules of \our is analogous to that of the incremental $T$.

In Figure \ref{fig:accuracyplot} we give an overview on the growing accuracy of \our during the training epochs of a DA experiment when using the residual transformer. In particular we show the accuracy plots for two runs (in red and blue) on the sources (the first three on the left) and the target (right).An increase in accuracy for the sources corresponds 
an analogous increase for the target, which indicates that \our is able to align the domains
with a clear effect on the target recognition performance.

\begin{figure*}[htb]
\centering
\includegraphics[width=0.95\textwidth]{residual}
\caption{Main blocks of our residual Transformer network. The blue block represent the input image data, while the red blocks are a sequence of Convolutional + Relu + Batch Normalization layers. The output of the two convolutional blocks are summed with the previous input. The number of kernels is fixed at 64 for the whole architecture until the last convolutional layer that brings the features back into 3 RGB channels (green block). }
\label{fig:transformer_residual}
\centering
\end{figure*}

\begin{table*}[hb!]
\centering
\caption{Ablation analysis on the experiment with three sources and target MNIST-M.
We turn on and off the different parts of the model: \textbf{T}= Residual Transformer, 
\textbf{E}= Entropy, \textbf{D}= Feature Domain Discriminator, \textbf{H}= Image Domain Discriminator. Analogous results are obtained when using the residual transformer.}
\begin{tabular}{ccccccccccc}
\hline
 %& \multicolumn{10}{c}{Mode}\\
 & T & T+E & T+D & D & D+E& T+H& T+D+H& T+E+H& T+D+E& T+D+E+H \\
 \hline
 DG & \multirow{2}{*}{61.7} & 61.7& 62.2& 53.0& 53.0& 58.7& 65.8& 58.7& 62.2&65.8\\
 DA &                       & 56.7& 65.4& 65.9& 75.1& 61.3& 62.5& 61.6& 82.9&87.6\\
\hline
\end{tabular}
\label{table:ablation3}
\end{table*}

\begin{figure*}[ht!]
\centering
\includegraphics[width=1\linewidth]{accuracies_v2}
\caption{Accuracy plots of our \our residual transformer training on SVHN as target, red and blue are two separate runs. The three plots on the left show the accuracy on the \textbf{sources}, the one on right accuracy on the \textbf{target}. Note how there is a strong correlation between the performance on the source and on the target. 
\label{fig:accuracyplot}
}
\end{figure*}

\textbf{Structure of $D$ and $H$} For the feature domain discriminator $D$ we used the same structured defined in \cite{Ganin:DANN:JMLR16}. The image domain discriminator $H$ is instead
built similarly to the main classification architecture, basically it is a copy of $F$ followed by $C$. Both $F$ and $C$ have the same structure presented in \cite{MDAN_ICLRW18}. Specifically $F$ is composed by three Convolutional $3 \times 3$ + ReLu + Maxpooling $2 \times 2$ blocks where the
number of convolutional maps grow from $64$ to $128$ and $256$. The classifier $C$ is instead 
composed by a  Convolutional $256 \times 3 \times 3$ layer  followed by two  ReLu + FullyConnected + Dropout blocks and ending with a last FullyConnected layer. The dimension
of the FullyConnected layers are respectively $2048$, $1024$, number of classes.

% $Conv$ $256 \times 3 \times 3$ - $ReLu$ - $FullyConnected$ $(2048)$ - $Dropout$ - 
% $ReLu$ - $FullyConnected$ $(1024)$ - $Dropout$ - $ReLu$ - $FullyConnected$ $(num_classes)$
% while the image domain discriminator is built similarly to the main classification architecture we used (basically a copy of F and C)
% More specifically, F and C were built as in [45], with F composed by:
% Conv 64 x 3x3 -> Relu -> MaxPool 2x2 -> Conv 128 x 3x3 -> Relu -> MaxPool 2x2 -> Conv 256 3x3 -> Relu -> MaxPool 2x2
% And C composed by:
% Conv 256 3x3 -> Relu -> FullyConnected (2048) -> Dropout -> Relu -> FullyConnected(1024) -> Dropout -> Relu -> FullyConnected(num_classes)

\textbf{Further Qualitative Results} For a further visual inspection of the results, we extended the qualitative analysis to the three sources experiments with SVHN as target. Figures \ref{fig:examples_best_svhn} and \ref{fig:tsne_svhn} show respectively the images produced by the transformer module of \our and the TSNE embedding of features extracted immediately before the final classifier. From both we can get to similar conclusions to those already elaborated in the main paper for the MNIST-M experiment.

 \begin{figure*}[tb]
     \centering
 \begin{subfigure}[b]{0.24\textwidth}
         \includegraphics[width=\textwidth]{combo_mnist_svhn}
         \caption{MNIST}
         \label{fig:mnist_adaptation_target_SVHN}
     \end{subfigure}
         \begin{subfigure}[b]{0.24\textwidth}
         \includegraphics[width=\textwidth]{combo_mnistM_svhn}
         \caption{MNIST-M}
         \label{fig:mnistM_adaptation_target_SVHN}
     \end{subfigure}
     \begin{subfigure}[b]{0.24\textwidth}
         \includegraphics[width=\textwidth]{combo_synth_svhn}
         \caption{SYNTH}
         \label{fig:synth_adaptation_target_SVHN}
     \end{subfigure}
      \begin{subfigure}[b]{0.24\textwidth}
         \includegraphics[width=\textwidth]{combo_svhn_svhn}
         \caption{SVHN}
         \label{fig:svhn_adaptation_target_SVHN}
     \end{subfigure}
 \caption{Examples of domain-agnostic digits generated by transformer block in the three source experiments with SVHN as target.
Top two rows show images produced in the DG setting by residual based (line $1$) and incremental based (line $2$) transformers. Line $3$ shows the original images and in the last two rows we display images produced by the residual (line $4$) and incremental transformers in the DA setting. As in the case with MNIST-M as target, images transformed with the residual architecture tend to preserve more of the original input. }
     \label{fig:examples_best_svhn}
     \vspace{-2mm}
 \end{figure*}
 
 \begin{figure*}[tb] 
 \centering
 \begin{subfigure}{0.3\textwidth}
 \includegraphics[width=0.9\linewidth]{deep_all_svhn} 
 \caption{combine sources}
 \end{subfigure}
 \begin{subfigure}{0.3\textwidth}
 \includegraphics[width=0.9\linewidth]{dg_svhn}
 \caption{DG \our}
 \end{subfigure}
 \begin{subfigure}{0.3\textwidth}
 \includegraphics[width=0.9\linewidth]{mda_svhn}
 \caption{DA \our}
 \end{subfigure}
 \caption{TSNE visualization of the classification features. Here SVHN is the target}
 \label{fig:tsne_svhn}
 \end{figure*}

\textbf{Further Quantitative Results} 
Table \ref{tab:resultsbis} is an extended version of the table presenting the three and four sources digits experiments in the main
paper. Here, besides the combine sources baseline implemented by us, we include also the reference results for the same baseline as reported in 
\cite{MDAN_ICLRW18} and \cite{cocktail_CVPR18}. We tried our best to replicate their base training protocol and network, still the
obtained results are slightly different from the published ones, so we report them here for completeness.
We also include in the table two other reference results. For the experiments with three sources, \cite{MDAN_ICLRW18} showed that 
choosing the source most related to the target and running DANN in this single source case provides higher recognition performance
that using all the sources together: these results are now in the left part of the table, line \emph{best single DANN}.
For the experiments with four sources, \cite{cocktail_CVPR18} indicated that running DANN separately on each source and then 
using the produced prediction in an average ensemble may provide an accuracy as good as DCTN in some setting: these results
appear now in the right part of the table, line \emph{separate DANN av.}.

As we have already discussed in the main paper, \our is defined for multi-source settings, but can still work reasonably 
well when dealing with a single source. To further analyze its behaviour we run an extra experiment on a single source setting
which involves objects instead of digits images. We consider as source the Synthetic Signs dataset \cite{Moiseev:2013}
and as target the German Traffic Signs Recognition Benchmark (GTSRB) \cite{gtsrb}. The first is a 
collection of $100$k images of common street signs obtained from Wikipedia and artificially transformed to simulate various 
imaging conditions, while the target consists of about $52$k cropped images of German traffic signs. Both
databases contain samples from 43 classes. Although this is an extreme condition for \our, it produces an accuracy of 95.7\%, 
just slightly worse than the recent 96.7\% result obtained with a GAN-based method in \cite{russo17sbadagan}.

For a more extensive evaluation on the effect of the number of sources on \our, we also ran experiments starting from the
four sources digits setting of the main paper, focusing in particular on the case with MNIST-M as target. We progressively
decreased the number of sources to two and three considering all the possible combinations of remaining sources. 
In the DG setting the average performance of \our on the three source cases is 59.7\%, practically equal to the result 60.0\% 
produced by the average combined sources baseline. Analogous results are observed for the two source case with an 
average accuracy for \our of 55.4\% with respect to 55.0\% of combined sources. As reference, in the four source case 
the results were 67.0\% for \our and 61.9\% for combined source. Thus, overall, a reduced number of sources means a 
drop in performance with equal effect on \our and the baseline.
For the DA setting the performance of \our shows a relatively smaller drop in performance when decreasing the source cardinality, 
passing from 85.3\% with four sources to an average of 82.3\% with three sources and 79.2\% with two sources, always 
maintaining a significant advantage over the combined sources baseline.

\begin{table*}[t]
%\centering
\caption{Extended edition of the classification accuracy results. \emph{On the left}: experiments with 3 sources. \emph{On the right}: experiments with 4 sources.
}
\label{tab:resultsbis}
\hspace{-0.9cm}
\begin{minipage}{.5\linewidth}
\centering \footnotesize
\begin{tabular}{@{}l@{~}l@{}c@{}c@{}c@{}c}
\hline
%\multicolumn{2}{c}{SVHN MnistM SYNTH $\rightarrow$ Mnist}   \\
  \multicolumn{2}{c}{ \multirow{3}{*}{Sources}}& SVHN & SVHN & MNIST-M&\multirow{4}{*}{Avg.}\\ [0.82ex]
  \multicolumn{2}{c}{ }& MNIST-M & MNIST & SYNTH\\ [0.82ex]
  \multicolumn{2}{c}{ }& SYNTH & SYNTH & MNIST\\ [0.82ex] \cline{2-5}
 \multicolumn{2}{c}{Target} & MNIST & MNIST-M & SVHN\\ \hline
 \multirow{5}{*}{DG}  & combine sources             &  98.7  & 62.6 & 69.5 & 76.9\\ 
   & combine sources  \cite{MDAN_ICLRW18}           &  92.8  & 56.1 & 81.4 & 76.8\\ 
 
 & MLDG \cite{MLDG_AAA18}   &  99.1  & 61.2 & 69.7 & 76.7\\\cline{2-6}
 & \our Residual            &  \textbf{99.2}  & 65.8 & 74.6 & 79.9 \\
& \our Incremental         &  99.1  & \textbf{66.3} & \textbf{76.4}  & \textbf{80.3}\\
 \hline \hline
 \multirow{5}{*}{DA} & combine sources &  98.7  & 62.6 & 69.5 & 76.9\\ 
  & best single DANN \cite{MDAN_ICLRW18}   & 96.7    &  59.1 &  81.8 & 79.2\\
  & combine DANN \cite{MDAN_ICLRW18}   &  92.5   & 65.1  &  77.6 & 78.4\\
  & MDAN \cite{MDAN_ICLRW18}   &  97.9   &  68.7 &  81.6 & 82.7\\ \cline{2-6}
  & \our Residual    &  99.2   &  87.6 &  84.1 & 90.3\\
  & \our Incremental    &  \textbf{99.3}   &  \textbf{88.5} &  \textbf{86.0} & \textbf{91.3}\\
\hline
\end{tabular}
\end{minipage}
\hspace{1.3cm}
\begin{minipage}{.3\linewidth}
\centering \footnotesize
\begin{tabular}{@{}l@{~}l@{}c@{}c@{}c}
\hline
  \multicolumn{2}{c}{ \multirow{4}{*}{Sources}}& SYNTH & SYNTH &\multirow{5}{*}{Avg.}\\
  \multicolumn{2}{c}{ }& MNIST & MNIST &\\
  \multicolumn{2}{c}{ }& MNIST-M & SVHN &\\
 \multicolumn{2}{c}{ }& USPS & USPS &\\ \cline{2-4}
 \multicolumn{2}{c}{Target} & SVHN & MNIST-M &\\ \hline
\multirow{5}{*}{DG}  & {combine sources}             &  73.2  &  61.9& 67.5\\ 
 & {combine sources} \cite{cocktail_CVPR18}            &  64.6  &  60.7& 62.7\\ 
 & MLDG \cite{MLDG_AAA18}     &  68.0  &  65.6 &  66.8 \\ \cline{2-5}
                     & \our  Residual             &  68.2  &  65.7 & 66.9 \\
                     & \our Incremental  &  \textbf{75.8}  &  \textbf{67.0} & \textbf{71.4} \\
 \hline \hline
 \multirow{5}{*}{DA} & {combine sources}             &  73.2  &  61.9 & 67.5\\ 
  & separate DANN av.\cite{cocktail_CVPR18}   &  61.4  &   71.1 & 66.3\\
  & combine DANN \cite{cocktail_CVPR18}   &  68.9   & 71.6  & 70.3 \\
  & DCTN \cite{cocktail_CVPR18}   &  77.5   &   70.9 & 74.2\\\cline{2-5}
  & \our Residual    & 82.3    &  84.1  & 83.2\\
  & \our Incremental    & \textbf{85.3}    &  \textbf{85.3}  & \textbf{85.3} \\
 \hline
\end{tabular}
\end{minipage}
\end{table*}
